# Supplementary material for: Simultaneous collapse of antiferroquadrupolar order and superconductivity in PrIr$_{2}$Zn$_{20}$ by nonhydrostatic pressure
Source: arXiv:2009.04708 source file (2020-09-11)
Supplement: Supplementary file 1 [file K_Umeo_PrIr2Zn20_Supplemental.pdf]

# Supplemental Material for "Simultaneous collapse of antiferroquadrupolar order and superconductivity in $PrIr_2Zn_{20}$ by non-hydrostatic pressure"

Kazunori Umeo[1], Riho Takikawa[2], Makoto Adachi[2], Keisuke T. Matsumoto[3], Takahiro Onimaru[2], and Toshiro Takabatake[2]

[1] *Department of Low Temperature Experiment, Integrated Experimental Support / Research Division, N-BARD, Hiroshima University, Higashi-Hiroshima, 739-8526, Japan*

[2]*Graduate School of Advanced Science and Engineering, Hiroshima University, Higashi-Hiroshima 739-8530, Japan*

[3]*Graduate School of Science and Engineering, Ehime University, Matsuyama 790-0826, Japan*

We describe here the measurements of the electrical resistivity $\rho(T)$ of $PrIr_2Zn_{20}$ under pressures with Daphne oil 7474 up to 2.1 GP and with Fluorinert 70/77=1:1 mixture pressures up to 9.6 GPa. We compare the pressure dependent hydrostaticity of the pressure transmitting media of argon, glycerol, and Fluorinert.

## 1. Electrical resistivity of $PrIr_2Zn_{20}$ under pressures up to 2.1 GPa applied with Daphne oil 7474

We used an ac four-terminal method and a piston-cylinder pressure cell. Daphne oil 7474 was used as pressure transmitting medium to apply hydrostatic pressure up to 3.7 GPa where it solidifies at room temperature. The pressure was estimated from the pressure dependence of the superconducting transition temperatures of a piece of lead placed in the cell. A commercial Cambridge Magnetic Refrigerator mFridge mF-ADR50 was used to cool the pressure cell down to 0.04 K.

Figure S1 shows the $\rho(T)$ data of $PrIr_2Zn_{20}$ under pressures up to 2.1 GPa. The superconducting transition temperature $T_c$ in $\rho(T)$ remains unchanged whereas the sharp drop at AFQ ordering temperature $T_Q$ shifts to higher temperatures. Both $T_c$ and $T_Q$ are plotted in Fig. 2(a).

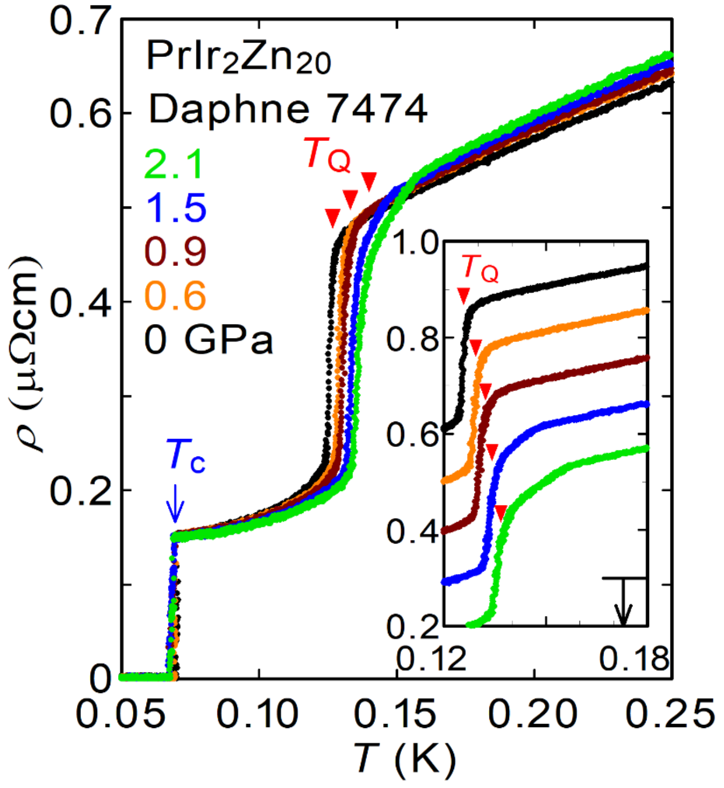


**Fig. S1.** Temperature dependence of the electrical resistivity $\rho(T)$ of $PrIr_2Zn_{20}$ under pressures up to 2.1 GPa applied with Daphne oil 7474. The triangles indicate the AFQ ordering temperature $T_Q$. The inset shows the data of $\rho(T)$ near $T_Q$, which are shifted downward by 0.1 μΩcm for clarity.

## 2. Electrical resistivity of $PrIr_2Zn_{20}$ under pressures applied with Fluorinert

We have measured $\rho(T)$ of $PrIr_2Zn_{20}$ under pressures up to 9 GPa using Fluorinert 70/77=1:1 mixture as a pressure transmitting medium. Since the Fluorinert solidifies at 1 GPa at room temperature, we expected that both $T_Q$ and $T_c$ simultaneously disappear above 1 GPa. Contrary to this expectation, we found that both AFQ order and superconductivity remain even at the maximal pressure of 9.6 GPa.

We employed an ac four-terminal method to measure the $\rho(T)$ under pressures using a piston-cylinder pressure cell for $P \leq 2.5$ GPa and an opposed-anvil pressure cell for $P \geq 3.2$ GPa. The pressure was estimated from the pressure dependence of the superconducting transition temperatures of a piece of lead placed in the cell. A commercial Cambridge Magnetic Refrigerator mFridge mF-ADR50 was used to cool the pressure cell down to 0.04 K.

As shown in Fig. S2 (a) and S2 (c), the step-like behavior in $\rho(T)$ of $PrIr_2Zn_{20}$ at $T_Q$ = 0.13 K becomes broader by applying pressure above 1 GPa that is the solidification pressure of Fluorinert. Even at the highest pressure of 2.5 GPa, however, the shoulder remains at around $T_Q$. The broadening of shoulder suggests a change from the long-range AFQ order to a sort of short-range AFQ order. On the other hand, the sharp superconducting transition in $\rho(T)$ at around 0.05 K has been observed at all pressures.

It is plausible that the non-hydrostatic pressure of 2.5 GPa applied by the piston-cylinder cell does not make sufficiently high uniaxial stress on the sample. Therefore, we have extended the pressure range up to 9.6 GPa using the opposed-anvil pressure cell. The results are shown in Fig. S2 (e). Upon applying pressure above 3.5 GPa, the shoulder at around $T_Q$ becomes broader while $T_c$ changes in a complex way. $T_c$ decreases from 0.066 K for $P$ = 3.5 GPa down to 0.049 K for $P$ = 5.8 GPa, where the resistivity does not fall to zero down to 0.035 K. Surprisingly, at 9.6 GPa, the broad shoulder at around $T_Q$ becomes larger than that for $P \leq 7.7$ GPa, and $T_c$ increases up to 0.07 K.

In Fig. S3, we summarize the pressure dependence of $T_Q$ and $T_c$ obtained by using Fluorinert 70/77 as a pressure transmitting medium. $T_Q$ was defined as the peak temperature of $d\rho/dT$ in Fig. S2 (b), (d), and (f). Additionally, we show the results obtained by using Daphne 7474, argon, and glycerol as pressure transmitting mediums in Fig. 2. $T_c(P)$ for Fluorinert is close to that for the hydrostatic condition using Daphne 7474 and argon. On the other hand, $T_Q(P)$ for $P$ >1 GPa becomes lower and higher, respectively, than those for Daphne 7474 and argon even at the same pressure. This fact suggests that $T_Q$ may vary according to the direction and magnitude of the uniaxial stress applied to the sample. In any case, the presence of AFQ order even at 9.6 GPa beyond the solidification pressure of 1 GPa for Fluorinert may be attributed to insufficient uniaxial stress to fully lift the degeneracy of the $\Gamma_3$ doublet. The pressure gradients will be discussed in the next section.

In summary, whenever $PrIr_2Zn_{20}$ is pressurized with Fluorinert up to 9.6 GPa, both the AFQ order and superconducting transition have been observed. This coexistence of AFQ order and superconductivity is consistent with the results under the hydrostatic condition produced by argon.

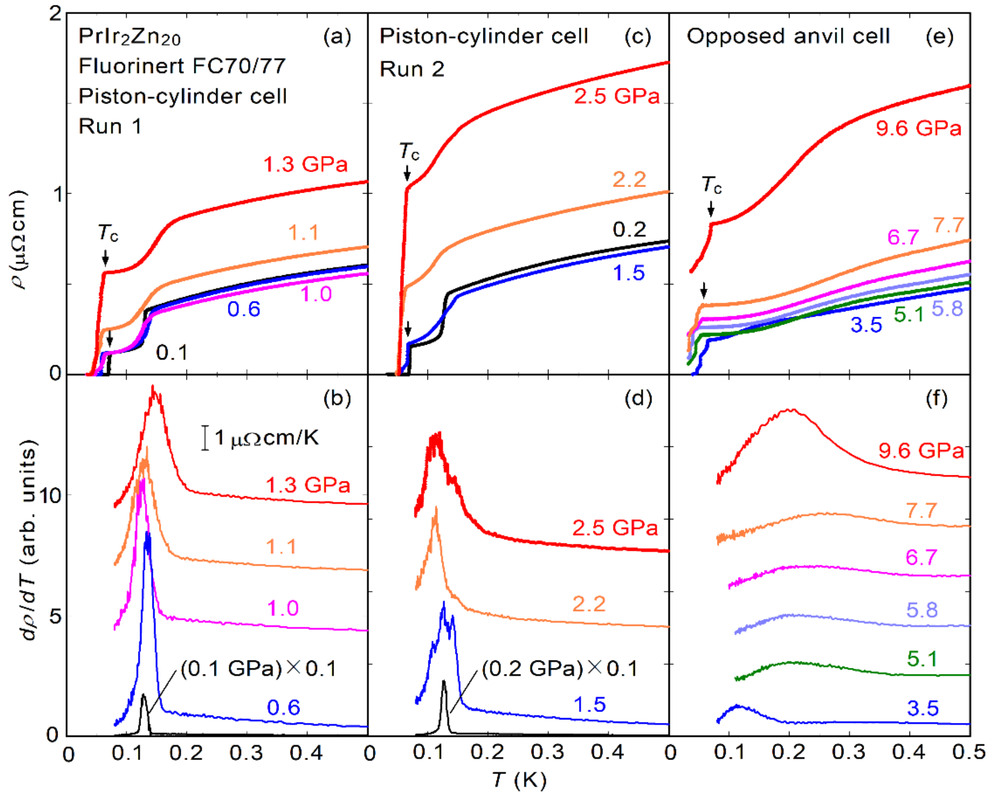


**Fig. S2.** (a) (c) (e) Temperature dependence of the electrical resistivity $\rho(T)$ under various pressures produced by the piston-cylinder cell and the opposed-anvil cell with Fluorinert 70/77 as a pressure transmitting medium. The data for (a) and (c) are measured by separate setups. (b) (d) (f) Temperature dependence of the derivative of $\rho(T)$, $d\rho/dT$, under various pressures for each data of (a), (c), and (e), respectively.

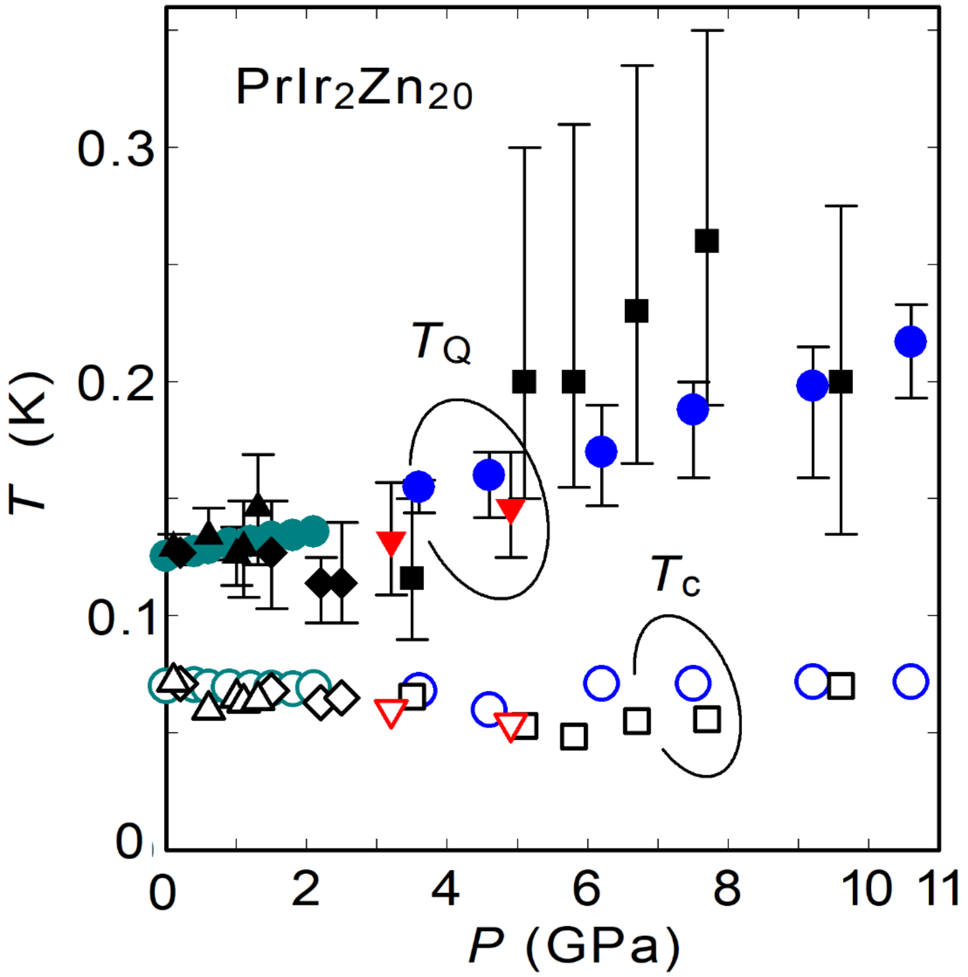


**Fig. S3.** Pressure dependences of the antiferroquadrupole ordering temperature $T_Q$ and superconducting transition temperature $T_c$ obtained by using the piston-cylinder cell (▲,△,◆,◇) and the opposed-anvil cell (■,□) with Fluorinert 70/77 as a pressure transmitting medium. The closed and open symbols denote $T_Q$ and $T_c$, respectively. $T_Q$ was defined as the peak temperature of $d\rho/dT$ in Fig. S2 (b), (d), and (f). The magnitude of error bar shows the full width at the half maximum of the peak of $d\rho/dT$ in Fig. S2 (b), (d), and (f). Additionally, we show the results obtained with Daphne 7474 and argon (●,○), and glycerol (▼, ▽) as pressure transmitting mediums from Fig. 2.

**3. Hydrostaticity of the pressure transmitting media**

In this section, we compare pressure dependence of the hydrostaticity of the pressure transmitting media of argon, glycerol, and Fluorinert. Figure S4 shows the pressure dependences of $\Delta P$ for each media estimated using the width of the superconducting transition of the Pb manometer for each medium. For glycerol, the data of $\Delta P$ for $P < 5$ GPa are small and close to those for argon. This result is consistent with the rather sharp drops in $\rho(T)$ at $T_Q$ and $T_c$ for glycerol up to 4.9 GPa as shown in Fig. 1.

For $P > 5$ GPa, however, the $\Delta P$ for glycerol increases significantly to 0.39 GPa at $P = 6.3$ GPa, which gives rise to the simultaneous disappearance of $T_Q$ and $T_c$. Note that $\Delta P$ for Fluorinert around 6 GPa is smaller than that for glycerol. Under this moderate $\Delta P$ at 6 GPa, broad drops in $\rho(T)$ were observed at both $T_Q$ and $T_c$.

For $P > 8$ GPa, $\Delta P$ for Fluorinert exceeds that for glycerol at 6.3 GPa as shown in Fig. S4. Even at 9.6 GPa for Fluorinert, however, broad anomalies in $\rho(T)$ remain at $T_Q$ and $T_c$ in the data of Fig. S2 (e). Next, we discuss this "inconsistency".

If the sample is pressurized by using the pressure transmitting medium such as argon and some liquid media with highly hydrostatic condition, the value of $\Delta P$ in the sample space is relatively small, and we expect that the $\Delta P$ measured by Pb manometer is close to $\Delta P_S$ along the sample. However, if the sample is pressurized by a solid pressure medium like Fluorinert for $P >$ 1 GPa, $\Delta P$ in the sample space would be larger than that for liquid medium. In that case, there should be some difference between $\Delta P$ along the Pb manometer and $\Delta P_S$ along the sample which are placed in a pressure cell as shown in Fig. S6. Furthermore, the deformation of the sample space at high pressures may cause complicated pressure distribution in the sample space. Therefore, the value $\Delta P$ for solid Fluorinert at $P > 8$ GPa cannot be compared with that for solid glycerol at $P > 6$ GPa. A similar situation occurred when the solid steatite was used as the pressure transmitting medium for resistivity measurements. Thereby, the absolute value of $\Delta P$ was found to be different for each setting [28].

In order to estimate $\Delta P_S$ along the sample, we have taken the temperature width of the drop of $\rho(T)$ at around $T_Q$. As mentioned in the main text, the AFQ order in $PrIr_2Zn_{20}$ is extremely sensitive to the uniformity of the pressure applied to the sample. We have estimated the transition width $\Delta T_Q$ of $\rho(T)$ at $T_Q$ which was defined as the full width at the half maximum of the peak of $d\rho(T)/dT$. As shown in Fig. S5, $\Delta T_Q$ for glycerol at $3 < P < 5$ GPa is comparable with that for argon but is smaller than that for Fluorinert. These results are consistent with the $P$ dependences of $\Delta P$ for $P < 6$ GPa in Fig. S4. Therefore, the transition width of $\rho(T)$ at around $T_Q$ is a good measure of the $\Delta P_S$ along the sample. Figure S5 shows that $\Delta T_Q$ for Fluorinert at $P > 5$ GPa is

saturated, in contrast to the continuous increase in $\Delta P$ shown in Fig. S4. The saturated behavior in $\Delta T_Q$ indicates the nearly constant value for $\Delta P_S$. Therefore, we expect that the $\Delta P_S$ for Fluorinert at $P$>5 GPa is smaller than that for glycerol at $P = 6.3$ GPa. If this is the case, it is not surprising that two anomalies remain at $T_c$ and $T_Q$ at 9.6 GPa for Fluorinert while they are completely suppressed at 6.3 GPa for glycerol.

Finally, we focus on $\Delta P_S$ for glycerol at 6.3 GPa. Above discussion means that the $\Delta P_S$ is not necessary to be equal to $\Delta P$= 0.39 GPa. Generally, the opposed anvil cell produces pressure gradient which increases from the center to the surrounding within the sample space [29]. As shown in Fig. S6, the $PrIr_2Zn_{20}$ sample is set near the center of the cell while the Pb manometer is set in the surrounding. Therefore, $\Delta P_S$ for solid glycerol may be smaller than the measured value of $\Delta P$= 0.39 GPa. In order to keep the AFQ order and superconductivity in $PrIr_2Zn_{20}$, $\Delta P_S$ needs to be smaller than 0.39 GPa. This condition helps us to set the uniaxial stress in the future.

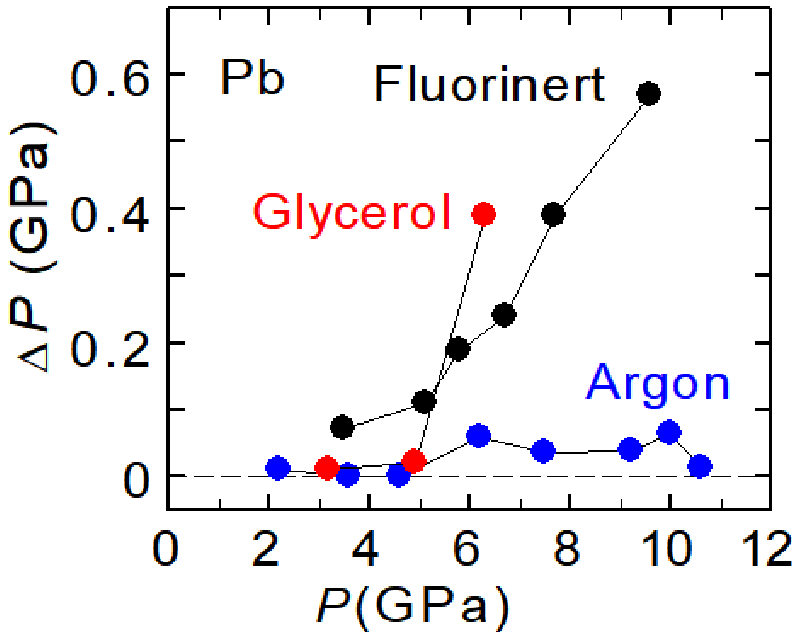


**Fig. S4.** Pressure dependences of the pressure gradient $\Delta P$ estimated from the temperature width of the superconducting transition of the Pb manometer for three pressure transmitting media of argon, glycerol, and Fluorinert 70/77.

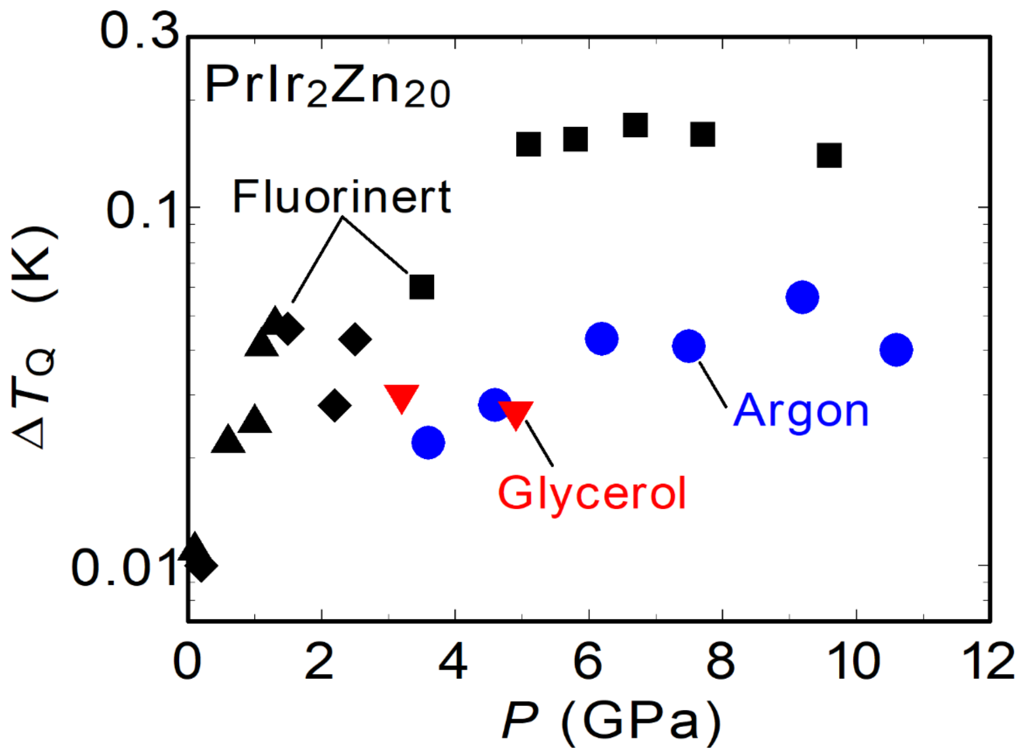


**Fig. S5.** Pressure dependences of the width of the antiferroquadrupole ordering temperature, $\Delta T_Q$ for argon (●), and glycerol (▼), and Fluorinert 70/77 (▲,◆, ■) as pressure transmitting media. The value of $\Delta T_Q$ is defined as the full width at the half maximum of the peak of $d\rho/dT$.

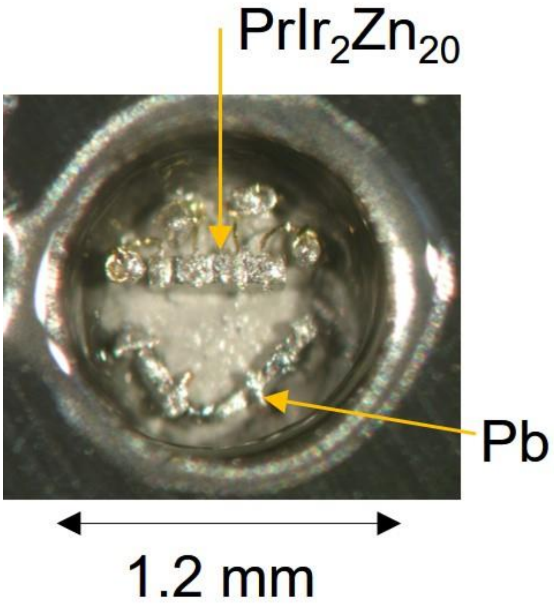


**Fig. S6.** Photograph of the sample space set with the $PrIr_2Zn_{20}$ sample and the Pb manometer in the opposed pressure cell when glycerol was used as pressure transmitting medium.
